# Supplementary material for: Neural Field Representations of Mobile Computational Photography
Source: arXiv:2508.05907 source file (2025-08-08)
Supplement: Supplementary file 1 [file definition.tex]

% formatting stuff

\definecolor{Gray}{rgb}{0.5,0.5,0.5}
\definecolor{darkblue}{rgb}{0,0,0.7}
\definecolor{orange}{rgb}{1,.5,0} % something readable but different from todo
\definecolor{red}{rgb}{1,0,0} % something readable but different from todo

% taken from https://designnavigator.daimler.com/Daimler_Color_System
\definecolor{dai_ligth_grey}{RGB}{230,230,230}
\definecolor{dai_ligth_grey20K}{RGB}{200,200,200}
\definecolor{dai_ligth_grey40K}{RGB}{158,158,158}
\definecolor{dai_ligth_grey60K}{RGB}{112,112,112}
\definecolor{dai_ligth_grey80K}{RGB}{68,68,68}
\definecolor{dai_petrol}{RGB}{0,103,127}
\definecolor{dai_petrol20K}{RGB}{0,86,106}
\definecolor{dai_petrol40K}{RGB}{0,67,85}
\definecolor{dai_petrol80}{RGB}{0,122,147}
\definecolor{dai_petrol60}{RGB}{80,151,171}
\definecolor{dai_petrol40}{RGB}{121,174,191}
\definecolor{dai_petrol20}{RGB}{166,202,216}
\definecolor{dai_deepred}{RGB}{113,24,12}
\definecolor{dai_deepred20K}{RGB}{90,19,10}
\definecolor{dai_deepred40K}{RGB}{68,14,7}
%\definecolor{violettblau}{cmyk}{0.9, 0.6, 0, 0}
\definecolor{rot}{RGB}{238, 28 35}
\definecolor{apfelgruen}{RGB}{140, 198, 62}
%\definecolor{gelb}{RGB}{255, 229, 0}
\definecolor{orange}{RGB}{244, 111, 33}
\definecolor{pink}{RGB}{237, 0, 140}
\definecolor{lila}{RGB}{128, 10, 145}
%\definecolor{hellgrau}{RGB}{224, 224, 224}
%\definecolor{mittelgrau}{RGB}{128, 128, 128}
%\definecolor{dunkelgrau}{RGB}{80,80,80}
\definecolor{anthrazit}{RGB}{19, 31, 31}

% \newcommand{\comment}[1]{{\small{\emph{\textcolor{Gray}{#1}}}}}

% \newcommand{\changed}[1]{{\textcolor{blue}{#1}}}

% dimensions
               % time coordinate
               % spatial coordinates in vectorized form
               % depth coordinate of volume

 % for writing
% for revision

% for comments
% for comments
% for comments

               % num pixels
               % num timesteps

%image formation

% notation for image formation

                % modulation on the PMD side
              % modulation of the light
                 % temporal period of the modulation
                % frequency of modulation
             % frequency of modulation harmonics
             % frequency of modulation harmonics of pmd camera
            % phase of PMD modulation
      % shorthand for freq/phase pair
              % #periods integrated over
               % geometric & photometric attenuation
  % space of all light paths

% regular modulation based cameras

% math stuff
         % fourier transform

 %Matrix
 %Vector
 %Identity matrix
 %Diagonalized matrix
 %Optimal point of an optimization
 %Convex conjugate
 %Operator
 %Minimize w.r.t.
 %Maximize w.r.t.

% notation for method
         		% Matrix basis
             % measurement matrix
             % measurement matrix element
            % measurement vector
            % measurement matrix
            % measurement matrix
                    % transient image
             % vectorized image

%

    % makes \addlegendimage available (typically only available within an
    % axis environment):
    \def\addlegendimage{\csname pgfplots@addlegendimage\endcsname}
