# Supplementary material for: Neural Field Representations of Mobile Computational Photography
Source: arXiv:2508.05907 source file (2025-08-08)
Supplement: Supplementary file 2 [file supplement_notation.tex]

%!TEX root = ../main.tex

 %revise

%\newcommand{\transportfun}[1]{f({#1})}

%\newcommand{\pois}{\textrm{Pois}}

% discrete measurement

% Functions

% Scalars

% Vectors

% Matrices

% Comparators
