# Supplementary material for: Neural Field Representations of Mobile Computational Photography
Source: arXiv:2508.05907 source file (2025-08-08)
Supplement: Supplementary file 3 [file 5_supplement.tex]

% \begin{figure}[t]
%     \centering
%     \includegraphics[width=\linewidth]{fig/gradient_loss.pdf}
%     \caption{Effect of gradient loss. (25x zoom)}
%     \label{fignsf:grad_loss}
%     \vspace{-1.5em}
% \end{figure}


% \vspace{1em}
% \section{Supplemental Document}
% Anything that doesn't make sense in the main paper body. For example, the following will definitely be in the supplemental:
% \begin{itemize}
%     \item Implementation details
%     \begin{itemize}
%         \item For example, we cut our long burst from Android to 42 frames for data regularity, but theoretically we could use more frames per capture.
%     \end{itemize}
%     \item Ablations
%     \begin{itemize}
%         \item with vs. without regularization
%         \item raw vs. tonemapped images
%         \item coarse to fine
%     \end{itemize}
%     \item Results/comparisons we couldn't fit in the previous step
%     \item Use as a dehazer if we didn't earlier? Maybe not if this gets too complicated, or we're stretched too thin. Keep in mind that NIR is pitched as a general plane separator, dehazing falls in its domain.
% \end{itemize}
% In this document we provide supporting material including additional results, implementation details, ablation experiments, and further analysis in support of the findings from the main text. We organize this material as follows:
% \begin{itemize}
% \itemsep0em 
%     \item Section~\ref{sec:implementation}: Data, training, and evaluation details.
%     \item Section~\ref{sec:ablation}: Additional ablation studies on manipulating network and encoding parameters.
%     \item Section~\ref{sec:additional_results}: Additional reconstruction results and examination of challenging imaging settings. 
%     \item Section~\ref{sec:synthetic}: Additional validation on simulated data with evaluation of motion estimates.
%     \item Section~\ref{sec:experiments}: Applications to depth and image matting. 
% \end{itemize}
% \setcounter{figure}{0}
% \renewcommand*{\theHfigure}{chX.\the\value{figure}}
% \setcounter{section}{0}
% \renewcommand*{\theHsection}{chX.\the\value{section}}
% \renewcommand\thesection{\Alph{section}}
% \section{Implementation Details}
% \label{sec:implementation}
% \noindent\textbf{Long-Burst Data.} We acquire long-burst data through a custom app built on the AVFoundation camera framework for iOS 16. While the vanilla AVFoundation framework offered a default method to capture burst or bracketed sequences, it was limited to only four frame sequences with significant overhead between captures, necessitating custom streaming code to save a longer continuous sequence of RAW data. A restriction we could not lift, however, is the inability to stream RAW captures from multiple cameras simultaneously. If this were possible, one could potentially use parallax and focus cues between two synchronized camera streams -- for example the wide and ultra-wide cameras -- to further improve reconstruction in the overlap of their fields of view. During capture, we record the following: Bayer CFA RAWs (42 frames $4032{\times}3024$px), processed RGB images (42 frames $1920{\times}1440$px), depth maps (42 frames $320{\times}240$px), frame timestamps, ISO, exposure time, brightness estimates, black level, white level, camera intrinsics, lens distortion tables, device acceleration estimates (${\smallsim}200$ measurements at 100Hz), device rotation estimates (${\smallsim}200$), and motion data timestamps (${\smallsim}200$). To preserve measured RAW values, we convert the single channel Bayer CFA images to three channel RGB volumes as shown in Fig.~\ref{fignsf:bayer_array}, linearly interpolating to fill missing values. To account for lens shading effects in bright scenes we also estimate a shade map with the help of a simple diffuser and uniform light source, illustrated in Fig.~\ref{fignsf:lens_shading}. We note that neglecting to compensate for lens shading can disrupt depth estimation in the corners of the image as matching pixels no longer have uniform brightness between frames.

% \begin{figure}[t!]
%     \centering
%     \includegraphics[width=\linewidth]{supp-fig/bayer_array.pdf}
%     \caption{The bayer color filter array on a camera sensor produces a spatially "mosaicked" RAW image, where each 2$\times$2 block contains a blue, red, and two green pixels. Rather than mix channel content to "demosaick" the image, we separate these channels into three planes and only linearly interpolate gaps between measured pixels, preserving the original RAW values.}
%     \label{fignsf:bayer_array}
%     \vspace{-1em}
% \end{figure}

% \begin{figure}[t!]
%     \centering
%     \includegraphics[width=\linewidth]{supp-fig/lens_shading.pdf}
%     \caption{(a) Lens shading is an effect caused by the geometry of the camera lens assembly, where regions close to the edge of the image sensor receive less total light than the center. (b) Camera manufacturers calibrate for this by capturing what should be a uniformly bright scene and (c) generating a \emph{shade map} to compensate for the observed fall-off in brightness in the image.}
%     \label{fignsf:lens_shading}
%     \vspace{-1em}
% \end{figure}


% \vspace{0.6em}
% \noindent\textbf{Training.} We sample 1024 points $(u,v)$ per iteration of training, projecting these to $42{\times}1024$ points in the image stack $I(u,v,\textsc{n})$, corresponding to 1024 points per frame. We perform 256 iterations per epoch, for 100 epochs of training with the Adam optimizer~\cite{kingma2014adam} with betas (0.9, 0.99) and epsilon $10^{-15}$. We exponentially decay learning rate during training with a factor of 0.98 per epoch. Training on a single Nvidia A100 takes approximately 15 minutes.

% \vspace{0.6em}
% \noindent\textbf{Evaluation.} To generate depth maps we sample $D(u,v)$ at a grid of $(\textsc{h},\textsc{w})\,{=}\,(1920,1440)$ points $(u,v)\,{\in}\,[0,1]$. To reduce noise introduced by the stochastic training process we median filter this result with kernel size 13 before visualization. For depth evaluation, we use relative absolute error \emph{L1-rel} and scale invariant error \emph{sc-inv} metrics, that is
% \begin{equation}
% \text{L1-rel}(d, \hat d) = \frac{1}{\textsc{h}\textsc{w}}\sum_{u.v} \frac{|d(u,v) - \hat d(u,v)|}{\hat d(u,v)}\nonumber ,
% \end{equation}
% \noindent and
% \begin{align}
% \text{sc-inv}(d, \hat d) &= \sqrt{\frac{1}{\textsc{h}\textsc{w}} \sum_{u,v} \delta(u,v)^2-\frac{1}{(\textsc{h}\textsc{w})^2}(\sum_{u,v} \hat \delta(u,v))^2}\nonumber\\
% \delta(u,v) &= \log(d(u,v)) - \log(\hat d(u,v)),\nonumber
% \end{align}
% which are often used in the monocular depth estimation literature~\cite{Ummenhofer2017} to compare approaches with varying scales and representations of depth. For methods such as MiDaS and RCVD we first convert inverse depth to depth before applying these metrics. We purposely avoid using photometric loss or reprojection error as comparison metrics~\cite{chugunov2022implicit} for similar arguments as discussed in Gao et al.~\cite{gao2022monocular}.
% \begin{equation}
%     \text{reprojection\_error}=\frac{1}{\textsc{h}\textsc{w}}\sum_{u,v,\textsc{n}} |I(u,v) - I(u^\textsc{n}, v^\textsc{n},\textsc{n})| \nonumber.
% \end{equation}
% Frames in a long-burst contain ${>}$90\% overlapping scene content, and so many non-physical solutions for depth will produce identical reprojection error as compared to more geometrically plausible depth maps. This is illustrated in Fig.~\ref{fignsf:reprojection_error}, where by ``tearing" the image -- compressing patches of similar colored pixels from the reference frame -- the non-physical depth incurs no additional photometric penalty, and so results in an identical reprojection error to a far more qualitatively plausible depth reconstruction.

% \section{Additional Ablation Experiments}
% \label{sec:ablation}
% \noindent\textbf{Encoding.} In this work we use the multiresolution hash encoding $\gamma_\textsc{d}$ to directly control what spatial information our implicit depth representation $f_\textsc{d}$ has access to during training. This in turn controls the scale of depth features we reconstruct, and presents a similar problem to choosing the scale factors in an image pyramid~\cite{adelson1984pyramid}. As we see in Fig.~\ref{fignsf:encoding_layers}, increasing the number of levels $L^{\gamma\textsc{d}}$ and effective max resolution $N_{max}^{\gamma\textsc{d}}$ increases the spatial frequency of reconstructed depth features. Scenes such as \emph{Branch} contain both high-frequency image and depth content, thin textured needles, and are best reconstructed by a fine resolution grid with $L^{\gamma\textsc{d}}=16$. The \emph{Desk Gourds}, however, have small image features in the patterns on the gourds, but relatively low-frequency depth features. Setting $L^{\gamma\textsc{d}}=16$ allows the network to overfit to these features and bleed image texture into the depth reconstruction. We select $L^{\gamma\textsc{d}}=8$ as a compromise between these imaging settings, but in practice, different scenes have different optimal encoding parameters for maximum reconstruction quality. We find hash table size $T^{\gamma\textsc{d}}$ significantly easier to tune, as choosing an overly large table size primarily affects model storage size, rather than reconstruction quality. We thus choose $T^{\gamma\textsc{d}}=2^{14}$, the smallest table size which does not lower the detail of depth reconstruction, as shown in Fig.~\ref{fignsf:encoding_hash}.

% \begin{figure}[t]
%     \centering
%     \includegraphics[width=\linewidth]{supp-fig/reprojection.pdf}
%     \caption{In this example both Depth A and B produce \emph{identical} reprojection error, but where Depth A models smooth geometry which warps the image between frames to model parallax, Depth B performs a brute-force mapping of individual pixels in the reference frame to points with similar values in the image stack.}
%     \label{fignsf:reprojection_error}
%     \vspace{-1em}
% \end{figure}


% \noindent\textbf{Depth Model.} The main adjustable parameter in our forward model is the plane regularization weight $\alpha_\textsc{p}$. This plane regularization affects depth reconstruction bidirectionally, regions with little parallax information are pulled towards the plane to remove spurious depth estimates, but in order to minimize depth offset, the plane is also pulled towards the reconstructed foreground objects. The effect of this can be seen in Fig.~\ref{fignsf:plane_weight}, where for very low $\alpha_\textsc{p}\,{\leq}\,10^{-5}$ this plane does not align with the foreground depth, and instead drifts into the background, causing a discontinuity in the reconstruction. Conversely, for large $\alpha_\textsc{p}\,{\geq}\,10^{-3}$, this regularization is so strong that the plane begins to cut into the foreground objects, flattening regions with low parallax information. We find $\alpha_\textsc{p}\,{=}\,10^{-4}$ to work well for a wide range of scenes, ``gluing'' the depth plane to the limit of reconstructed objects. We note that in scenes such as \emph{Desk Gourds}, and as we will see later with synthetic data, this plane accurately reconstructs the real geometry of the background. However, for many settings it is more akin to a \emph{segmentation mask} than depth, designating the area which we cannot reconstruct using parallax information.

% \begin{figure*}[t!]
%     \centering
%     \includegraphics[width=\linewidth]{supp-fig/encoding_layers.pdf}
%     \caption{Ablation study on the effect of the number of levels $L^{\gamma\textsc{d}}$, and effective max resolution $N_{max}^{\gamma\textsc{d}}$, in the multiresolution hash encoding $\gamma_\textsc{d}$ on reconstruction. Here, given a scale factor of $\sqrt{2}$ between levels, $L^{\gamma\textsc{d}}=2,4,6,8,16$ correspond to $N_{max}^{\gamma\textsc{d}}=16,32,128,2048$. The qualitatively best reconstructions are highlighted with a dashed border.}
%     \label{fignsf:encoding_layers}
% \end{figure*}

% \begin{figure*}[t!]
%     \centering
%     \includegraphics[width=\linewidth]{supp-fig/encoding_hash.pdf}
%     \caption{Ablation study on the effect of hash table size $T^{\gamma\textsc{d}}$ on reconstruction quality. Selected $T^{\gamma\textsc{d}}$ is highlighted with a dashed border.}
%     \label{fignsf:encoding_hash}
% \end{figure*}

% \begin{figure*}[htp!]
% \vspace*{-1.2em}
%     \centering
%     \includegraphics[width=\linewidth]{supp-fig/plane_weight.pdf}
%     \caption{Ablation study on the effects of regularization weight $\alpha_\textsc{p}$ on reconstruction quality. Selected $\alpha_\textsc{p}$ highlighted with a dashed border.}
%     \label{fignsf:plane_weight}
% \bigskip
%     \includegraphics[width=\linewidth]{supp-fig/control_points.pdf}
%     \caption{Ablation study on the effect of the number of chosen control points $N^\textsc{t}_c\,{=}\,N^\textsc{r}_c$ on reconstruction quality, with image reconstructions $I(u,v)$ and estimated motion paths plotted below. The selected number of control points is highlighted with a dashed border.}
%     \label{fignsf:control_points}
% \bigskip

%     \includegraphics[width=\linewidth]{supp-fig/difficult_scenes.pdf}
%     \caption{Depth reconstruction results for a set of challenging imaging scenarios. Not visible is the large motion of leaves in the \emph{Dynamic} scene, captured during high wind. Areas of interest are highlighted with a dashed border.}
%     \vspace*{-0.5em}
%     \label{fignsf:difficult_scenes}
% \end{figure*}

% \begin{figure*}[htp!]
%     \centering
%     \includegraphics[width=\linewidth]{supp-fig/small_motion.pdf}
%     \caption{Depth reconstruction results for long-bursts captured with normal (approximately 5 millimeter maximum effective stereo baseline) and minimal (on the scale of a millimeter) hand shake motion. Major depth artifacts are highlighted with a dashed border.}
%     \label{fignsf:small_motion}
% \end{figure*}

% \begin{figure}[t]
%     \centering
%     \includegraphics[width=\linewidth]{supp-fig/non-lambertian.pdf}
%     \caption{(a) Objects which reflect local scene content, in this example a mirror-finish copper pot reflecting the carpet around it, can completely break view consistency assumptions used for depth reconstruction. Even small view angle changes result in light paths which sample completely inconsistent colors in the surrounding environment. (b) In contrast, objects with specularities caused by a light source at effectively infinity, in this example polished ceramic reflecting sunlight, do not fully break view consistency.}
%     \label{fignsf:non-lambertian}
%     \vspace{-1em}
% \end{figure}

% \noindent\textbf{Motion Model.} We use a B\'ezier curve model to represent translation between frames, as natural hand-tremor draws a continuous low-velocity path during capture. By limiting the number of control points $N_c$ in this model we can enforce smoothness constraints on this motion, the effects of which are illustrated in Fig.~\ref{fignsf:control_points}. Not surprisingly, using too few control points does not allow us to faithfully model camera motion and results in blurry image reconstruction and inconsistent depth estimates. We thus choose the smallest number of control points which leads to successful image and depth reconstruction. We note that while for \emph{Desk Gourds} reconstruction succeeded with $N_c=42$, for many scenes setting $N_c\,{\geq}\,42$ leads to \emph{very unstable} training as the over-defined motion model can generate erratic high-velocity motion between frames.

% \begin{figure*}[htp!]
%     \centering
%     \includegraphics[width=\linewidth]{supp-fig/results_supp.pdf}
%     \caption{Reconstruction on 7 additional scenes for our method and a mix of learned, purely multi-view, and mixed depth estimation methods. Given the mix of depth representations, results are re-scaled by minimizing relative mean square error.}
%     \label{fignsf:results_supp}
% \end{figure*}

% %\newpage
% \section{Additional Reconstruction Results}
% \noindent\textbf{Challenging Imaging Scenarios.} Given the fundamental building blocks of our approach, namely that it performs multi-view depth estimation through ray reprojection, some scenes will naturally be more difficult to reconstruct than others. As shown in Fig.~\ref{fignsf:difficult_scenes}, each of these scenarios presents its own set of challenges and direction of study. In the \emph{Dynamic} scene, we fail to reconstruct accurate depth for the majority of the plant leaves as they undergo deformation far larger than the parallax effects we observe in the long-burst. Our forward model has no way to model this deformation, and it is notoriously difficult to separate the effects of object motion from camera motion. The \emph{Textureless} and \emph{Distant} scenes present two sides of a similar problem, insufficient parallax information. While we are able to reconstruct the plant in \emph{Textureless}, the textureless planter provides no multi-view information from which to estimate depth except for along its edges, which we can track relative to the motion of the background. The church in \emph{Distant} is so far from the camera that it exhibits only fractions of pixel in disparity over the entire long-burst. In both these scenarios we need a mechanism to aggregate information in image space to make up for the lack of parallax. In \emph{Textureless} this would be in-painting the planters depth based on its edges, and in \emph{Distant} we would need to look at the deformation of larger image patches to estimate sub-pixel motion. The \emph{Thin Structures} reconstruction is partially successful, as in the foreground region we are able to track and reconstruct the depth of the thin orange mesh, but breaks down when it begins to overlap with the traffic cone. We suspect this is because our forward model is a single-layer RGB-D representation, with no explicit way to model for occlusions. In the region of the traffic cone is has to decide between reconstructing the cone or the mesh in front of it in the long-burst $I(u,v,\textsc{n})$ data, not both. Here, a layered depth representation could potentially solve this, but greatly increases the complexity of the problem as we would now need to learn an alpha map for each frame $\textsc{n}$ to sample these layers. For the \emph{Very High Dynamic Range} scene, we have specular reflections three orders of magnitude brighter than the shadowed portions of the statue. While using the fixed auto exposure and ISO settings we are able to reconstruct a large portion of the statue body with our RAW data. To reconstruct all the regions of the scene, including the dimly-lit body, our model could potentially be augmented to incorporate bracketed image data with varying exposure, similar to Mildenhall et al.~\cite{mildenhall2022nerf}, and perform joint HDR image volume and depth reconstruction. The \emph{Lens Blur} scene shows a loss in reconstruction quality due to portions of the scene being blurred by a shallow depth of field from the camera. Depth-from-defocus cues~\cite{xiong1993depth} could potentially help regularize reconstruction in these areas which are otherwise devoid of fine image features. Lastly, the \emph{Translucent} and \emph{Highly Reflective} settings both violate view consistency. Namely, changes in pixel colors can no longer be attributed solely to parallax or camera motion, and can be caused by seeing through or around the objects. We further discuss the reconstruction of non-lambertian objects in the next section.

% \noindent\textbf{Non-Lambertian Reconstruction.}  While we focus on the reconstruction of primarily lambertian scenes -- matte, diffusely-reflective objects -- non-lambertian scenes provide an interesting set of both imaging challenges and opportunities. We first divide this setting into two categories: \emph{local reflections} and \emph{distant light sources}, illustrated in Fig.~\ref{fignsf:non-lambertian}. In the first setting, sampled light paths and colors can drastically change for even small view variations. As photometric matching tries to match reflected content, which does not follow the parallax motion of the reflective object itself, this produces erroneous depth estimates for objects such as the copper pot in Fig.~\ref{fignsf:non-lambertian} (a). With a distant light source, however, small changes in view angle result in the same apparent specularities as the path from the camera center to the illuminator remains connected. These specularities thus act as image texture, and exhibit the same parallax effects as the surface of the object. As seen in Fig.~\ref{fignsf:non-lambertian} (b) and the \emph{Tiger} scene, this does not disrupt depth reconstruction. This finding, that specularities from distant light sources act as object texture and local reflections do not, points towards an avenue of work in lighting separation and reflection removal. Regions which do not fit a static RGB-D model and incur large photometric penalties regardless of their depth, could be separated into view-dependent texture plus reflection components for later manipulation.

% \noindent\textbf{Small Camera Motion.}  As hand shake is a naturally random process, long-burst captures have varying effective stereo baseline. While on average we can expect 5-6 millimeters of baseline~\cite{chugunov2022implicit}, if we are unlucky -- e.g. the user is not taking a breath and is rigidly holding the phone with two hands close to their body -- this motion can be as small as a millimeter. Illustrated in Fig.~\ref{fignsf:small_motion}, we see how our end--to-end camera pose estimation still converges in the minimal baseline setting, and how we are able to produce useable -- albeit blurrier -- depth estimates. This is in contrast to HNDR~\cite{chugunov2022implicit}, which uses the imperfect ARKit pose estimates for reprojection and produces major artifacts because of it, mapping incorrect pixel matches to spurious depths solutions. This demonstrates the value of continuous pose refinement, as mobile SLAM algorithms and COLMAP~\cite{schonberger2016structure} \emph{do not produce ground truth poses}.

% \noindent\textbf{Additional Results.} \label{sec:additional_results}
% Fig.~\ref{fignsf:results_supp} provides additional qualitative comparisons of our proposed approach to a wide set of baseline methods. This includes the four target objects used to demonstrate object reconstruction in the main text, prefixed with \emph{Obj-}. The visualizations also reflect the challenges in evaluating methods purely from depth maps, as geometric inconsistencies that are apparent in the mesh projections -- such as the distorted arms of \emph{Obj-Ganesha} -- are much harder to identify in these 2D visualizations. In addition to these objects, we include 3 scenes \emph{Leopardy, Bush, and Houseplant}, which demonstrate successful reconstruction with deceptive image features, small depth features, and large field of view respectively. Of particular note is how we are able to reconstruct the needles of the \emph{Bush} scene and individual leaves of \emph{Houseplant}, where other methods blend features at different depth levels together. 

% \section{Synthetic Evaluation}
% \label{sec:synthetic}
% \vspace{0.6em} \noindent\textbf{Setup.} To further validate our approach we use the high-fidelity structured light object scans we acquired for quantitative evaluation to generate simulated long-burst captures. Illustrated in Fig~\ref{fignsf:synthetic_results}, we apply a Voronoi color texture to the surface of these meshes, and place them in front of a tilted background plane with an outdoor image texture. We add depth-of-field effects and match camera intrinsics to our real captures -- using the ARKit poses captured by the software from Chugunov et al.~\cite{chugunov2022implicit} to generate realistic hand tremor motion paths -- and render frames at 16-bit color depth with Blender's Eevee engine. This synthetic data allows us to not only validate the fidelity of our object reconstructions, but also our estimated camera motion paths, for which we cannot otherwise get ground truth during ordinary captures.
% \\
% %
% \begin{figure*}[ht!]
%     \centering
%     \includegraphics[width=\linewidth]{supp-fig/synthetic_results.pdf}
%     \caption{Depth reconstruction and motion estimation results for a set of simulated textured objects with realistic hand-tremor motion. Motion estimates are re-normalized and overlaid to demonstrate the accuracy in estimated camera trajectory to ground truth data.}
%     \label{fignsf:synthetic_results}
% \end{figure*}

% \noindent\textbf{Assessment on Synthetic Data.} We find that for this synthetic data -- in the absence of noise, lighting changes, and other imaging non-idealities -- we are able to recover nearly ground truth reconstructions of both the objects and background planes. This supports our plane plus offset depth model, which fits the simple plane to the out-of-focus background content instead of generating spurious depth estimates for regions without reliable parallax information. Though the colorful object textures make single-view depth estimation visually difficult, as illustrated by artifacts in the MiDaS reconstructions, these high-contrast cues allow our method to reconstruct even tiny features such as the tusks of the \emph{Synth-Ganesha}. This validates that even with small camera motion, given sufficient image texture we converge to geometrically correct solutions. In Fig.~\ref{fignsf:synthetic_results} we also see how the camera motion estimates converge close to ground truth as our method jointly refines depth and camera trajectory estimates during training. 

% \section{Depth and Image Matting}
% \label{sec:experiments}
% \noindent\textbf{Forward Model Decomposition.} In the proposed plane plus offset depth model, regions that do not generate sufficient parallax information are pulled towards the plane by the regularization term $R$. While we cannot recover meaningful depth from multiview in these regions, they prove \emph{useful for scene segmentation and editing}. Illustrated in Fig.~\ref{fignsf:editting} (a), by masking what parts of the image produce negligible depth offset, we are able to cleanly segment the tiger statue in \emph{Scene A} from its background. In Fig.~\ref{fignsf:editting} (b) we then superimpose this masked image over \emph{Scene B}, a separately captured tree-covered street. We run \emph{Scene B} through MiDaS to hallucinate the depth of the background trees, and overlay this with our geometrically-estimated depth of the tiger to produce a fused depth representation. In this way we leverage multiview information where we have it, and learned image priors where we do not. In \textbfFig.~\ref{fignsf:editting} (c) we see an advantage of using this plane separation technique for segmentation over depth thresholding. As the floor under the dragon figure extends both in front of and behind the figure itself, setting a depth cutoff will always either miss a part of the figure, or include the area around it. Whereas as our plane here represents the depth of the floor, we can threshold the depth offset just like in Fig.~\ref{fignsf:editting} (a) to recover a \emph{high-quality mask of the object}. Thanks to being based on depth rather than image features, this approach has no problems with the visual ambiguity of the dragon and its background, which both contain high-frequency black and white textures.

% \newpage
% \begin{figure*}[t!]
%     \centering
%     \includegraphics[width=\linewidth]{supp-fig/editting.pdf}
%     \caption{Image and Depth Matting. Example of scene editing enabled by our plane plus offset forward model. We can (a) threshold the depth offset component $d(u,v) - d_\textsc{p}$ to recover a mask of the object in focus and then (b) superimpose it over a new scene. (c) This works even for visually ambiguous scenes where simple depth thresholding fails.}
%     \vspace*{5in}
%     \label{fignsf:editting}
% \end{figure*}
	

% % \end{document}
